# Supplementary material for: HeadCraft: Modeling High-Detail Shape Variations for Animated 3DMMs
Source: arXiv:2312.14140 source file (2025-01-31)
Supplement: Supplementary file 1 [file fitting_w_and_noise_compn.tex]

% \vspace{-0.2cm}
\begin{table}[t!]
    \centering
    \setlength{\tabcolsep}{0pt}
    \begin{tabular}{ccccc}
    $\mathcal{W}+$ & $\mathcal{W}+$ \& Noise & \hspace{0.3cm} & $\mathcal{W}+$ & $\mathcal{W}+$ \& Noise \\
    \includegraphics[width=0.11\textwidth,trim={4cm 1cm 0.5cm 1cm},clip]{} 
    & \includegraphics[width=0.11\textwidth,trim={4cm 1cm 0.5cm 1cm},clip]{}         
    & \hspace{0.4cm}
    & \includegraphics[width=0.11\textwidth,trim={4cm 1cm 0.5cm 1cm},clip]{}  
    & \includegraphics[width=0.11\textwidth,trim={4cm 1cm 0.5cm 1cm},clip]{} 
    \\
    \includegraphics[width=0.11\textwidth,trim={4cm 1cm 0.5cm 1cm},clip]{} 
    & \includegraphics[width=0.11\textwidth,trim={4cm 1cm 0.5cm 1cm},clip]{}         
    &  \hspace{0.4cm}
    & \includegraphics[width=0.11\textwidth,trim={4cm 1cm 0.5cm 1cm},clip]{}  
    & \includegraphics[width=0.11\textwidth,trim={4cm 1cm 0.5cm 1cm},clip]{} 
    \end{tabular}
    \captionof{figure}{
    The result of fitting the $w \in \mathcal{W}+$ latent code and subsequently the StyleGAN noise to a registered complete UV map.
    }
    \label{fig:fitting_w_and_noise_compn}
    \vspace{-0.4cm}
\end{table}
