# Supplementary material for: HeadCraft: Modeling High-Detail Shape Variations for Animated 3DMMs
Source: arXiv:2312.14140 source file (2025-01-31)
Supplement: Supplementary file 2 [file seam.tex]

\begin{table}[h!]
    \centering
    \setlength{\tabcolsep}{0pt}
    \begin{tabular}{cp{0.3cm}c}
    Standard UV & \hspace{0.3cm} & Custom UV \\
    \includegraphics[width=0.4\linewidth,trim={1cm 1cm 0.5cm 1cm},clip]{supp_fig/seam/standard_seam.jpg} 
    & \hspace{0.3cm}
    & \includegraphics[width=0.4\linewidth,trim={1cm 1cm 0.5cm 0cm},clip]{supp_fig/seam/new_seam.jpg} \\
    \end{tabular}
    \vspace{-0.2cm}
    \captionof{figure}{
    Demonstration of the custom UV seam annotation.
    \textit{Standard UV} corresponds to the UV space shipped with the FLAME model.
    \textit{Custom UV} stands for the handcrafted layout employed in our pipeline.
    This layout simplifies learning sophisticated shape variations such as long hair in a consistent way.
    }
    \label{fig:seam}
\end{table}
